# Supplementary material for: Specify and Edit: Overcoming Ambiguity in Text-Based Image Editing
Source: arXiv:2407.20232 source file (2024-07-29)
Supplement: Supplementary file 1 [file supp_intro.tex]

\makeatletter
\NewDocumentCommand{\MakeTitleInner}{ +m +m +m }{
    \newpage%
    \null%
    \vskip 2em%
    \begin{center}%
        \let \footnote \thanks
        {\LARGE #1 \par}%
        \vskip 1.5em%
        {%
            \large
            \lineskip .5em%
            \begin{tabular}[t]{c}%
                #2%
            \end{tabular}\par%
        }%
        \vskip 1em%
        {\large #3}%
    \end{center}%
    \par
    \vskip 1.5em%
}
\NewDocumentCommand{\MakeTitle}{ +m +m +m }{%
    \begingroup
        \renewcommand\thefootnote{\@fnsymbol\c@footnote}%
        \def\@makefnmark{\rlap{\@textsuperscript{\normalfont\@thefnmark}}}%
        \long\def\@makefntext##1{\parindent 1em\noindent
            \hb@xt@1.8em{%
                \hss\@textsuperscript{\normalfont\@thefnmark}%
            }##1%
        }%
        \if@twocolumn
            \ifnum \col@number=\@ne
                \MakeTitleInner{#1}{#2}{#3}
            \else
                \twocolumn[\MakeTitleInner{#1}{#2}{#3}]%
            \fi
        \else
            \newpage
            \global\@topnum\z@   %
            \MakeTitleInner{#1}{#2}{#3}
        \fi
        \thispagestyle{plain}\@thanks
    \endgroup
    \setcounter{footnote}{0}%
}
\makeatother

\clearpage

\setcounter{section}{0}
\definecolor{cvprblue}{rgb}{0.21,0.49,0.74}

\MakeTitle{Specify and Edit: Overcoming Ambiguity in Text-Based Image Editing\\
\textit{Appendix
}}{}{}

In the main paper, we present \methodname, a novel zero-shot pipeline for instruction-based diffusion models, used to boost performance on ambiguous instructions. In this appendix, we propose additional information to complement our paper. We discuss limitations in Section~\ref{sec:supp-limitations}. Then, in Section~\ref{sec:supp-prompts} we report the LLM prompts used for each task. Finally, in Section~\ref{sec:supp-exp} we 
provide additional results, including new experiments and qualitative evaluations.
